# Supplementary material for: Ultra-Stable Ferrimagnetic Second-Order Topological Insulator in 2D Metal-Organic Framework
Source: arXiv:2502.15257 source file (2025-02-21)
Supplement: Supplementary file 1 [file Supporting_Information.pdf]

*Supporting Information for*

# Ultra-Stable Ferrimagnetic Second-Order Topological Insulator in 2D Metal-Organic Framework

Meijun Wang, Yong-An Zhong, Lei Jin\*, Ying Liu, Xuefang Dai, Guodong Liu and Xiaoming Zhang\*

*State Key Laboratory of Reliability and Intelligence of Electrical Equipment, and School of Materials Science and Engineering, Hebei University of Technology, Tianjin 300130, China*

**I. The monolayer Cr(pyz)<sub>2</sub> during AIMD simulations at 300 K**

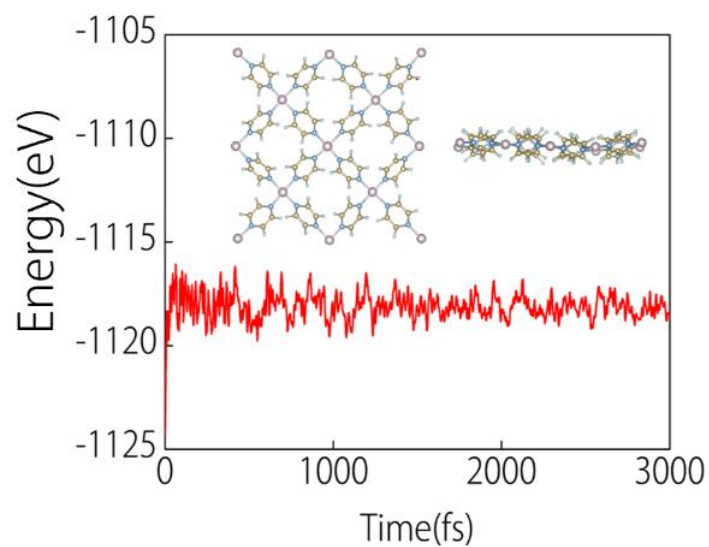

**Figure S1.** Total potential energy fluctuations of the monolayer Cr(pyz)<sub>2</sub> during *ab initio* molecular dynamics (AIMD) simulations at 300 K; the inset shows the final state of the structure.

## II. PDOS of monolayer Cr(pyz)<sub>2</sub>

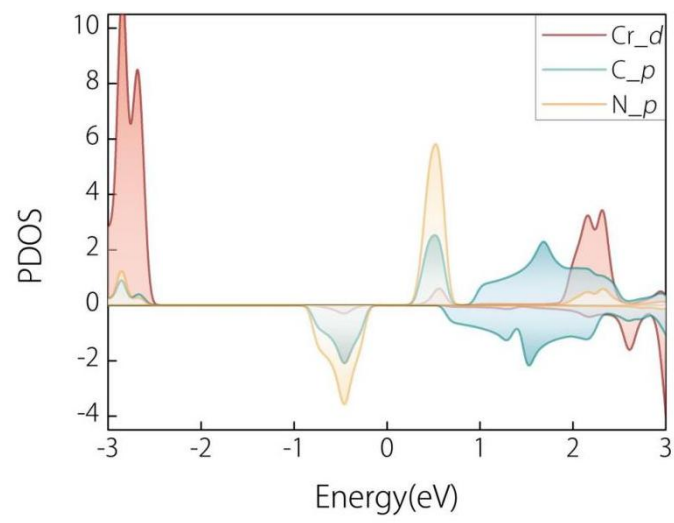

**Figure S2.** Projected density of states (PDOS) of Cr(pyz)<sub>2</sub>.

### III. Band structures and energy gap values of monolayer Cr(pyz)<sub>2</sub> under different $U$ values

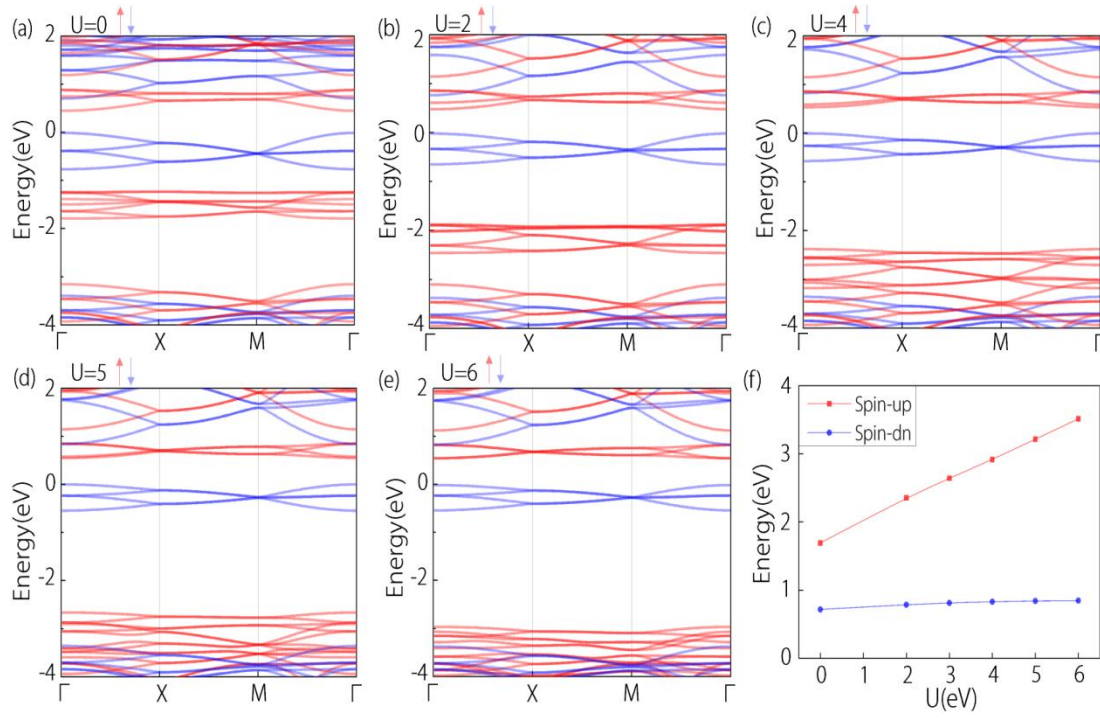

**Figure S3.** The band structures of monolayer Cr(pyz)<sub>2</sub> when the  $U$  values are chosen as (a) 0, (b) 2, (c) 4, (d) 5, and (e) 6 eV. (f) shows the changes of band gap in the spin-up and spin-down channels, respectively.

**IV. Edge states in two spin channels, the energy spectrum and the spatial distribution of the edge and bulk modes for spin-down channel**

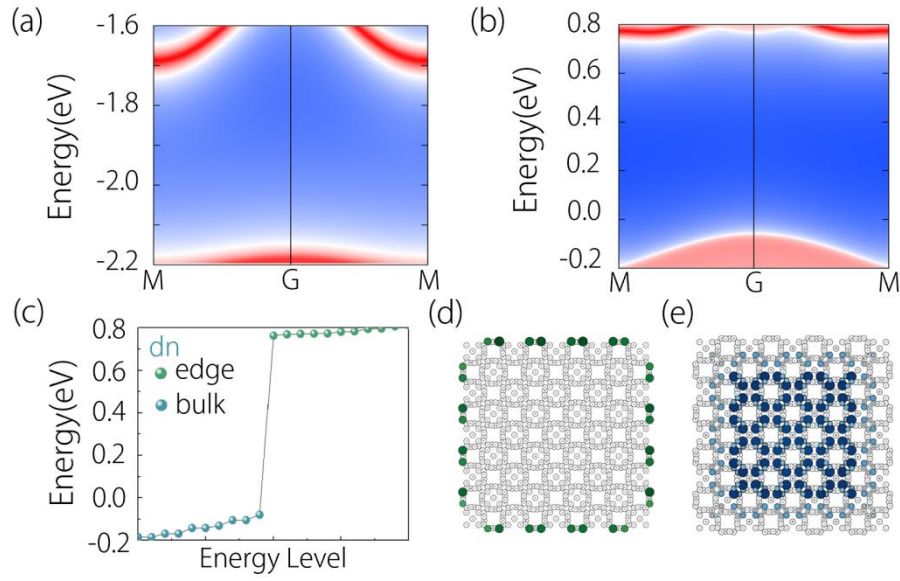

**Figure S4.** (a) and (b) are the edge states of the spin-up and spin-down channels, respectively. (c) shows the energy spectrum for the square disk of the spin-down channel. (d) and (e) The spatial distribution of edge and bulk modes for  $\text{Cr}(\text{pyz})_2$  disks, corresponding to the green and blue dots in (c), respectively.
